# Supplementary material for: PlaceRAN: Optimal Placement of Virtualized Network Functions in the Next-generation Radio Access Networks
Source: arXiv:2102.13192 source file (2021-03-29)
Supplement: Supplementary file 1 [file Additional.tex]

\begin{savenotes}
\begin{table}[!h]
    \caption{Additional Setup for Fibre and RAN}
    \label{tab:additional}%
    \centering{ {
        \begin{tabular}{|l|c|c|c|c|c|}
        \hline
        \multicolumn{1}{|c|}{Fibre Inputs} & \multicolumn{5}{c|}{Latency (ms)$^{1}$}  \\ \hline
        
        \rowcolor[HTML]{cdd5e4} WDM Optic & \multicolumn{5}{c|}{0.010625} \\ \hline
      
        WDM Electric  & \multicolumn{5}{c| }{0.0005} \\ \hline
      
       \rowcolor[HTML]{cdd5e4} Fiber ??? & \multicolumn{5}{c|}{0.000005} \\ \hline \hline
      
       \multicolumn{1}{|c|}{RAN Inputs} & Channel & YYY & MIMO & PRB & SPB \\ 
       \multicolumn{1}{|c|}{} & (MHz) &  & (layers) &  & (KHz) \\ \hline
      
      \rowcolor[HTML]{cdd5e4} gNB profile 1 & 40 & 32T32R & 8 & 216 & 15  \\ \hline
      
      gNB profile 2 & 100 & 64T64R & 8 & 132 & 60 \\ \hline 
      
%      \hline
      
%       \multicolumn{2}{|c|}{RU Inputs} & F1 & F3 & Rand1 & Rand2 \\ \hline
       
%       \rowcolor[HTML]{cdd5e4} \multicolumn{2}{|l|}{Number of RUs} & 1 & 3 & 0 to 1 & 0 to 3  \\ \hline
    
       \end{tabular}
    } }
\end{table}
\end{savenotes}
